# Supplementary material for: Autonomous discovery of new structure-plausibility laws for explainable and rapid crystal diagnosis and screening
Source: arXiv:2609.01209 source file (2026-11-18)
Supplement: Supplementary file 1 [file si-xr.tex]

\makeatletter
\expandafter\gdef\csname r@si-note:s1\endcsname{{S1}{3}{Autonomous discovery protocol and its audit trail}{section.1}{}}
\expandafter\gdef\csname r@si-s1.1-what-was-autonomous\endcsname{{S1.1}{3}{What was autonomous}{subsection.1.1}{}}
\expandafter\gdef\csname r@si-s1.2-the-audit-trail\endcsname{{S1.2}{3}{How the discovery trail was audited}{subsection.1.2}{}}
\expandafter\gdef\csname r@si-s1.3-run-statistics\endcsname{{S1.3}{3}{Scale and outcomes of the autonomous search}{subsection.1.3}{}}
\expandafter\gdef\csname r@si-s1.4-a-caveat-on-what-this-does-and-does-not-demonstrate\endcsname{{S1.4}{4}{The audit catches documented errors, not unknown ones}{subsection.1.4}{}}
\expandafter\gdef\csname r@si-note:s2\endcsname{{S2}{4}{Data sources, licences and the analysis set}{section.2}{}}
\expandafter\gdef\csname r@si-s2.1-sources\endcsname{{S2.1}{4}{Sources}{subsection.2.1}{}}
\expandafter\gdef\csname r@si-sifig:ledger\endcsname{{S1}{5}{Refuted-claim ledger}{figure.caption.2}{}}
\expandafter\gdef\csname r@si-sifig:modes\endcsname{{S2}{6}{Refutations grouped by failure mode}{figure.caption.3}{}}
\expandafter\gdef\csname r@si-s2.2-the-analysis-funnel\endcsname{{S2.2}{6}{How structures entered the analysis}{subsection.2.2}{}}
\expandafter\gdef\csname r@si-s2.3-why-omat24-was-screened-out\endcsname{{S2.3}{6}{Why OMat24 was screened out}{subsection.2.3}{}}
\expandafter\gdef\csname r@si-s2.4-the-64-that-cannot-be-judged\endcsname{{S2.4}{6}{Formal-charge assignment limits the evaluable population}{subsection.2.4}{}}
\expandafter\gdef\csname r@si-note:s3\endcsname{{S3}{6}{Feature definitions}{section.3}{}}
\expandafter\gdef\csname r@si-s3.1-oxidation-states\endcsname{{S3.1}{7}{Oxidation states}{subsection.3.1}{}}
\expandafter\gdef\csname r@si-s3.1b-lookup\endcsname{{S3.2}{7}{Fixed radius and bond-valence lookups make parameter choices reproducible}{subsection.3.2}{}}
\expandafter\gdef\csname r@si-s3.2-neighbour-algorithm-robustness\endcsname{{S3.3}{8}{Neighbour-algorithm robustness}{subsection.3.3}{}}
\expandafter\gdef\csname r@si-s3.3-missing-values\endcsname{{S3.4}{8}{Missing values and minimum feature availability}{subsection.3.4}{}}
\expandafter\gdef\csname r@si-note:s4\endcsname{{S4}{8}{Searching for simple crystal-plausibility laws}{section.4}{}}
\expandafter\gdef\csname r@si-s4.1-objective\endcsname{{S4.1}{8}{The search balances satisfaction against damage detection}{subsection.4.1}{}}
\expandafter\gdef\csname r@si-s4.2-two-defects-found-in-our-own-search\endcsname{{S4.2}{8}{Executable checks exposed two search defects}{subsection.4.2}{}}
\expandafter\gdef\csname r@si-s4.3-search-configuration\endcsname{{S4.3}{8}{A fixed search grid limits how much the search can adapt to the data}{subsection.4.3}{}}
\expandafter\gdef\csname r@si-s4.4-scoring-formulas\endcsname{{S4.4}{9}{Composition controls prevent misleading cross-database comparisons}{subsection.4.4}{}}
\expandafter\gdef\csname r@si-sifig:ranking-data\endcsname{{S3}{9}{Ranking-data scale and composition}{figure.caption.4}{}}
\expandafter\gdef\csname r@si-note:s5\endcsname{{S5}{9}{Composition-preserving perturbations isolate structural failure modes}{section.5}{}}
\expandafter\gdef\csname r@si-sifig:perclass\endcsname{{S4}{10}{Per-class damage detection}{figure.caption.5}{}}
\expandafter\gdef\csname r@si-note:s6\endcsname{{S6}{10}{The eleven refuted conclusions}{section.6}{}}
\expandafter\gdef\csname r@si-s6.1-r8-an-identity-mistaken-for-evidence\endcsname{{S6.1}{10}{R8: an identity mistaken for evidence}{subsection.6.1}{}}
\expandafter\gdef\csname r@si-sifig:amplitude\endcsname{{S5}{11}{Damage detection versus perturbation amplitude}{figure.caption.6}{}}
\expandafter\gdef\csname r@si-s6.2-r10-a-lesson-recorded-then-repeated\endcsname{{S6.2}{11}{R10: a lesson recorded, then repeated}{subsection.6.2}{}}
\expandafter\gdef\csname r@si-note:s7\endcsname{{S7}{11}{Which feature families improve damage detection}{section.7}{}}
\expandafter\gdef\csname r@si-note:s8\endcsname{{S8}{12}{Split discipline, revisions and the reserve split-labelling error}{section.8}{}}
\expandafter\gdef\csname r@si-sifig:split-consistency\endcsname{{S6}{13}{Discovery and held-out splits}{figure.caption.7}{}}
\expandafter\gdef\csname r@si-sifig:pris-composition-holdout\endcsname{{S7}{13}{Frozen PRIS performance on compositions unseen during discovery}{figure.caption.8}{}}
\expandafter\gdef\csname r@si-note:s9\endcsname{{S9}{14}{Reproducing the analysis}{section.9}{}}
\expandafter\gdef\csname r@si-note:s10\endcsname{{S10}{14}{Exact search does not remove omitted-class sensitivity within the tested shallow-tree space}{section.10}{}}
\expandafter\gdef\csname r@si-note:s11\endcsname{{S11}{15}{What a one-sided criterion misses, and the condition that repairs it}{section.11}{}}
\expandafter\gdef\csname r@si-note:s12\endcsname{{S12}{16}{Exact perturbation operators used in D1--D5}{section.12}{}}
\expandafter\gdef\csname r@si-sifig:threshold\endcsname{{S8}{17}{Contact-threshold sensitivity}{figure.caption.9}{}}
\expandafter\gdef\csname r@si-sifig:band-grid\endcsname{{S9}{17}{Two-dimensional contact-band scan}{figure.caption.10}{}}
\expandafter\gdef\csname r@si-sifig:unguarded\endcsname{{S10}{18}{Law sets and an unconditional two-sided band}{figure.caption.11}{}}
\expandafter\gdef\csname r@si-sifig:chemistry\endcsname{{S11}{18}{Performance by anion family}{figure.caption.12}{}}
\expandafter\gdef\csname r@si-sifig:dft-e1-landscape\endcsname{{S12}{19}{First-principles energy landscape behind the contact thresholds}{figure.caption.13}{}}
\expandafter\gdef\csname r@si-sifig:loko\endcsname{{S13}{19}{Leave-one-perturbation-out tests}{figure.caption.14}{}}
\expandafter\gdef\csname r@si-sifig:validation-boundary-omission\endcsname{{S14}{20}{Conditional contact thresholds and leave-one-damage-class-out evaluation}{figure.caption.15}{}}
\expandafter\gdef\csname r@si-note:s13\endcsname{{S13}{20}{Composition-grouped ranking separates decision rate from accuracy}{section.13}{}}
\expandafter\gdef\csname r@si-note:s14\endcsname{{S14}{21}{Supplementary figure conventions and source data}{section.14}{}}
\expandafter\gdef\csname r@si-note:s15\endcsname{{S15}{21}{PRIS-derived synthesis score for composition-held-out ranking}{section.15}{}}
\expandafter\gdef\csname r@si-sifig:pss-coefficient-stability\endcsname{{S15}{23}{Coefficient stability of the fitted synthesis score}{figure.caption.16}{}}
\expandafter\gdef\csname r@si-sifig:pss-term-correlation\endcsname{{S16}{23}{Correlation among the terms of the fitted synthesis score}{figure.caption.17}{}}
\expandafter\gdef\csname r@si-note:pu-transfer\endcsname{{S16}{24}{PRIS and PSS are linearly correlated with predicted synthesizability across two PU models}{section.16}{}}
\expandafter\gdef\csname r@si-sifig:l4-contribution\endcsname{{S17}{24}{Law-wise attribution of Set~4 screening}{figure.caption.18}{}}
\expandafter\gdef\csname r@si-sifig:pu-model-performance\endcsname{{S18}{25}{Validation performance of the two PU models}{figure.caption.19}{}}
\expandafter\gdef\csname r@si-sifig:polymorph-ranking\endcsname{{S19}{26}{Decision boundaries in same-composition polymorph ranking}{figure.caption.20}{}}
\expandafter\gdef\csname r@si-sifig:dft-e4-bulk\endcsname{{S20}{27}{Property screen against first-principles bulk moduli}{figure.caption.21}{}}
\expandafter\gdef\csname r@si-sifig:dft-e4-composition\endcsname{{S21}{27}{Composition and symmetry of the relaxed design candidates}{figure.caption.22}{}}
\expandafter\gdef\csname r@si-note:s17\endcsname{{S17}{28}{Extending the plausibility sequence with structural simplicity and bond valence}{section.17}{}}
\expandafter\gdef\csname r@si-si-note:s17\endcsname{{S17}{28}{Extending the plausibility sequence with structural simplicity and bond valence}{section.17}{}}
\expandafter\gdef\csname r@si-si-note:s17-gnome\endcsname{{S17.7}{30}{The distinct-site law exposes excess site complexity in a public generative release}{subsection.17.7}{}}
\expandafter\gdef\csname r@si-s17.x-realworld\endcsname{{S17.11}{33}{The laws return no verdict outside their domain and detect anomalies in the evaluable falsified depositions}{subsection.17.11}{}}
\expandafter\gdef\csname r@si-s17.x-incumbents-scored\endcsname{{S17.13}{33}{Composition and structure screens detect different failures}{subsection.17.13}{}}
\expandafter\gdef\csname r@si-note:s18\endcsname{{S18}{34}{Robustness and implementation details}{section.18}{}}
\expandafter\gdef\csname r@si-sifig:energy-phonon-record\endcsname{{S22}{37}{Energy, phonons and experimental record}{figure.caption.23}{}}
\expandafter\gdef\csname r@si-sifig:charge-coverage\endcsname{{S23}{38}{Coverage of charge-dependent PRIS laws in GNoME}{figure.caption.24}{}}
\expandafter\gdef\csname r@si-sifig:dft-e3-paired\endcsname{{S24}{38}{Machine-learned relaxation energies against first principles}{figure.caption.25}{}}
\expandafter\gdef\csname r@si-sifig:dft-e2-ordering\endcsname{{S25}{39}{Ordering energies behind the GNoME attribution}{figure.caption.26}{}}
\expandafter\gdef\csname r@si-note:s19\endcsname{{S19}{40}{Shared evaluation procedure across pre-registered analyses}{section.19}{}}
\expandafter\gdef\csname r@si-note:dft\endcsname{{S20}{40}{Pre-registered first-principles tests of four learned quantities}{section.20}{}}
\expandafter\gdef\csname r@si-note:methods-ext\endcsname{{S21}{41}{Extended Methods}{section.21}{}}
\makeatother
